# Supplementary material for: Nested Session Types
Source: arXiv:2010.06482 source file (2020-12-09)
Supplement: Supplementary file 1 [file appendix.tex]

\appendix

\section{Appendix}
\label{sec:appendix}

\begin{proof}[\autoref{thm:equiv-grammars}]
	For the direct implication, assume that 
	$\llparenthesis A\rrparenthesis \not\sim_{\mathcal{S}}
	\llparenthesis B\rrparenthesis$.
	It means that the traces are different.
	Let $w \in \m{trace}(\llparenthesis A\rrparenthesis)$
	and $w \not\in \m{trace}(\llparenthesis B\rrparenthesis)$
	and let $w_0$ be the greatest prefix that occurs in
	$ \m{trace}(\llparenthesis B\rrparenthesis)$.
	Either $w_0$ is a maximal trace of $\llparenthesis B\rrparenthesis$, 
	or we have 
	$\llparenthesis A\rrparenthesis \xrightarrow{w_0}\llparenthesis A'\rrparenthesis$
	and 
	$\llparenthesis B\rrparenthesis \xrightarrow{w_0}\llparenthesis B'\rrparenthesis$,
	with 
	$\llparenthesis A'\rrparenthesis \xrightarrow{a_1}\llparenthesis A''\rrparenthesis$
	and
	$\llparenthesis B'\rrparenthesis \xrightarrow{a_2}\llparenthesis B''\rrparenthesis$,
	where $a_1\neq a_2$. In both cases, with a 
	simple case analysis on
	the definition of the translation $\tau$, we conclude that 
	$A' \not\equiv B'$ and so $A \not\equiv B$.
	For the reciprocal implication, assume that 
	$\llparenthesis A\rrparenthesis \sim_{\mathcal{S}}	\llparenthesis B\rrparenthesis$.
	Consider the relation 
	\begin{equation*}
		\mathcal{R} = \{(A_0,B_0) \mid \m{trace}_{\mathcal{S}}(\llparenthesis A_0\rrparenthesis) = \m{trace}_{\mathcal{S}}(\llparenthesis B_0\rrparenthesis)\}\subseteq  \mi{Type} \times \mi{Type}.
	\end{equation*}
	Obviously, $(A,B)\in \mathcal{R}$. To prove that $\mathcal{R}$ is
	a type bisimulation, let $(A_0, B_0)\in \mathcal{R}$ and proceed 
	by case analysis on $A_0$ and $B_0$. We sketch a few cases for $A_0$.
	The other cases are analogous.
	
	Case $\unfold{A_0} = \ichoice{\ell \colon A_\ell}_{\ell\in L}$.
	In this case we have 
	$\llparenthesis A_0\rrparenthesis\xrightarrow{\ichoiceop \ell} \llparenthesis A_\ell\rrparenthesis$.
	Since, by hypothesis, the traces coincide,
	$\m{trace}(\llparenthesis A_0\rrparenthesis) = \m{trace}(\llparenthesis B_0\rrparenthesis)$,
	we have
	$\llparenthesis B_0\rrparenthesis\xrightarrow{\ichoiceop \ell} \llparenthesis B_\ell\rrparenthesis$ and,
	thus, $\unfold{B_0} = \ichoice{\ell \colon B_\ell}_{\ell\in L}$.
	Moreover, Jan\v{c}ar~\cite{Jancar10} proves that
	$\m{trace}(\llparenthesis A_\ell\rrparenthesis) = \m{trace}(\llparenthesis B_\ell\rrparenthesis)$.
	Hence, $(A_\ell,B_\ell)\in \mathcal{R}$.
	
	Case $\unfold{A_0} = \texists{\alpha}A_1$.
	We have
	$\llparenthesis A_0\rrparenthesis\xrightarrow{\exists} 
	\llparenthesis A_1[X/\alpha]\rrparenthesis$,
	for some type name $X$ for which
	$(\llparenthesis X \rrparenthesis \xrightarrow{\delta} \bot)\in \mathcal{S}$.
	For the same reason as in the previous case,
	$\llparenthesis B_0\rrparenthesis\xrightarrow{\exists} \llparenthesis B_1[X'/\beta]\rrparenthesis$
	and $\unfold{B_0} = \texists{\beta}B_1$. 
	By Jan{\v{c}}ar's observation, we also have
	$\m{trace}(\llparenthesis A_1[X/\alpha]\rrparenthesis) = \m{trace}(\llparenthesis B_1[X'/\beta]\rrparenthesis)$.
	Now let $C$ be any closed type. 
	To conclude that $(A_1[C/\alpha], B_1[C/\beta])\in \mathcal{R}$, we 
	need to verify that 
	$\m{trace}(\llparenthesis A_1[C/\alpha]\rrparenthesis) = 
	\m{trace}(\llparenthesis B_1[C/\beta]\rrparenthesis) $.
	If $\alpha$ does not occur in $A_1$ and $\beta$ does not occur in 
	$B_1$, then 
	\begin{equation*}
		\m{trace}(\llparenthesis A_1[C/\alpha]\rrparenthesis)
    	= \m{trace}(\llparenthesis A_1[X/\alpha]\rrparenthesis) 
    	= \m{trace}(\llparenthesis B_1[X'/\beta]\rrparenthesis) 
    	= \m{trace}(\llparenthesis B_1[C/\beta]\rrparenthesis).
	\end{equation*}
	If $\alpha$ occurs in $A_1$ and $\beta$ does not occur in $B_1$,
	or vice-versa, we could easily prove that 
	$\m{trace}_{\mathcal{S}}(\llparenthesis A_0\rrparenthesis) \neq \m{trace}_{\mathcal{S}}(\llparenthesis B_0\rrparenthesis)$.
	Hence, assume that $\alpha$ occurs in $A_1$, $\beta$ occurs in $B_1$,
	and let $\delta'$ be s.t. $(\llparenthesis X' \rrparenthesis \xrightarrow{\delta'} \bot)\in \mathcal{S}$.
	Note that, since 
	\begin{equation*}
	\begin{array}{ll}
		\m{trace}(\llparenthesis A_1[X/\alpha]\rrparenthesis) 
	= &\{w\cdot \delta \mid \llparenthesis A_1[X/\alpha]\rrparenthesis\xrightarrow{w} \llparenthesis X \rrparenthesis \}\\
	\m{trace}(\llparenthesis B_1[X'/\beta]\rrparenthesis)
	=  &\{w'\cdot \delta' \mid \llparenthesis B_1[X'/\beta]\rrparenthesis\xrightarrow{w'} \llparenthesis X'\rrparenthesis\}
	\end{array}
	\end{equation*}
	and $\m{trace}(\llparenthesis A_1[X/\alpha]\rrparenthesis) = \m{trace}(\llparenthesis B_1[X'/\beta]\rrparenthesis)$, we have
	$\delta=\delta'$. We also have 
	\begin{equation}
		\{w \mid \llparenthesis A_1[X/\alpha]\rrparenthesis\xrightarrow{w} \llparenthesis X \rrparenthesis \} = \{w' \mid \llparenthesis B_1[X'/\beta]\rrparenthesis\xrightarrow{w'} \llparenthesis X' \rrparenthesis \}:
	\end{equation}	
	for this, observe that the only way to trigger action 
	$\delta$ in $\llparenthesis B_1[X'/\beta]\rrparenthesis$ is by reaching $X'$; if we had $w\cdot \delta\in \m{trace}(\llparenthesis A_1[X/\alpha]\rrparenthesis)$
	such that $\llparenthesis A_1[X/\alpha]\rrparenthesis\xrightarrow{w} \llparenthesis X \rrparenthesis$
	but $\llparenthesis B_1[X'/\beta]\rrparenthesis\not\xrightarrow{w} \llparenthesis X'\rrparenthesis$, 
	then $w\cdot \delta\not \in \m{trace}(\llparenthesis B_1[X'/\beta]\rrparenthesis)$.
	Conclude that
	$\m{trace}(\llparenthesis A_1[C/\alpha]\rrparenthesis) = 
	\m{trace}(\llparenthesis B_1[C/\beta]\rrparenthesis) $ by noticing that:	
	\begin{equation*}
	\begin{array}{ll}
		\m{trace}(\llparenthesis A_1[C/\alpha]\rrparenthesis) 
	= &\m{trace}(\llparenthesis A_1[X/\alpha]\rrparenthesis\,\cup \\
	&\{w\cdot v \mid \llparenthesis A_1[X/\alpha]\rrparenthesis\xrightarrow{w} \llparenthesis X\rrparenthesis, v\in \m{trace}(\llparenthesis C\rrparenthesis) \}\\
	\m{trace}(\llparenthesis B_1[C/\beta]\rrparenthesis)
	= &\m{trace}(\llparenthesis B_1[X'/\beta]\rrparenthesis\,\cup\\
	& \{w\cdot v \mid \llparenthesis B_1[X'/\alpha]\rrparenthesis\xrightarrow{w} \llparenthesis X'\rrparenthesis,
	v\in \m{trace}(\llparenthesis C\rrparenthesis) \}
	\end{array}
	\end{equation*}

	Case $\unfold{A_0} = \one$. In this case,
	$\m{trace}_{\mathcal{S}}(\llparenthesis A_0\rrparenthesis) = \m{trace}_{\mathcal{S}}(\bot) = \emptyset $.
	Since $B_0$ is a closed type and 
	$\m{trace}_{\mathcal{S}}(\llparenthesis A_0\rrparenthesis) = \m{trace}_{\mathcal{S}}(\llparenthesis B_0\rrparenthesis)$
	and the types are contractive,
	we have $\unfold{B_0} = \one$.
\end{proof}

\begin{proof}[\autoref{thm:tpeq_sound}]
  Given a derivation $\mathcal{D}_0$ of $\vars_0 \semi \cdot \vdash A_0 \equiv B_0$,
  construct $\mathcal{S}(\mathcal{D}_0)$ and define relation $\rel_0$ as follows:
  \[
    \rel_0 = \{(A[\sigma], B[\sigma]) \mid \clo{\vars}{A \equiv B}
    \in \mathcal{S}(\mathcal{D}_0)\;\mbox{and}\;\sigma\;\mbox{over}\;\vars \label{bis:1}\}
  \]
  Consider $\rel$ to be the \emph{reflexive transitive closure} of $\rel_0$.
  We prove that $\rel$ is a type bisimulation. Then our theorem follows
  since the closure
  $\clo{\vars_0}{A_0 \equiv B_0} \in \mathcal{S}(\mathcal{D}_0)$.
  % \frank{please verify}

  Consider $(A[\sigma], B[\sigma]) \in \rel$ where
  $\clo{\vars}{A \equiv B} \in \mathcal{S}(\mathcal{D}_0)$ for
  some $\sigma$ over $\vars$. We case analyze on the structure of $A[\sigma]$.

  Consider the case where $A = \ichoice{\ell : A_\ell}_{\ell \in L}$. Since $A$ and $B$
  are both structural, $B = \ichoice{\ell : B_\ell}_{\ell \in L}$
  (due to internal naming). Since
  $\clo{\vars}{A \equiv B} \in \mathcal{S}(\mathcal{D}_0)$, by definition of
  $\mathcal{S}(\mathcal{D}_0)$, we get
  $\clo{\vars}{A_\ell \equiv B_\ell} \in \mathcal{S}(\mathcal{D}_0)$ for all
  $\ell \in L$. By the definition of $\rel$, we get that
  $(A_\ell[\sigma], B_\ell[\sigma]) \in \rel$. Also,
  $A[\sigma] = \ichoice{\ell : A_\ell[\sigma]}_{\ell \in L}$ and similarly,
  $B[\sigma] = \ichoice{\ell : B_\ell[\sigma]}_{\ell \in L}$.  Hence, $\rel$ satisfies the
  appropriate closure condition for a type bisimulation.

  If $A = \alpha$, then $B = \alpha$ since the last applied rule must be $\m{var}$.
  Then $A[\sigma] = B[\sigma]$ and since $\rel$ contains $(A[\sigma], B[\sigma])$
  for all $\sigma$ over $\vars$, we get that $\rel$ satisfies the closure
  conditions for a bisimulation.

  Next, consider the case where $A = \texists{\alpha} A'$. Since $A$ and $B$ are both
  structural, $B = \texists{\beta} B'$. Since $\clo{\vars}{A \equiv B}
  \in \mathcal{S}(\mathcal{D}_0)$, we get that $\clo{\vars,\gamma}
  {A'[\gamma/\alpha] \equiv B'[\gamma/\alpha]} \in \mathcal{S}(\mathcal{D}_0)$.
  Thus we obtain that $(A'[\sigma, C/\gamma], B'[\sigma,  C/\gamma]) \in \rel$
  for all $C \in \mi{Type}$ and the closure condition is satisfied.

  % Thus, for any substitution $\sigma$ over $\vars, k$ such that
  % $\cdot \proves \cons[\sigma]$, we get that $(A'[k/m][\sigma], B'[k/n][\sigma])
  % \in \rel$. Since $\sigma$ is over $\vars, k$, we know that $k$ is substituted
  % over a closed term, and since $\cons$ does not mention $k$, we know that $k$
  % can be substituted with any closed term. Thus, $\forall i \in \mathbb{N}$,
  % $(A'[i/k][k/m][\sigma], B'[i/k][k/n][\sigma]) \in \rel$. Thus, $\rel$ is a type
  % simulation.

  Finally, consider the case $A = V_1 \indv{A_1}$ and $B = V_2 \indv{A_2}$. If the last applied
  rule is $\m{expd}$, then $\clo{\vars}{A \equiv B} \in \mathcal{S}(\mathcal{D}_0)$,
  and thus $(A[\sigma], B[\sigma]) \in \rel$, satisfying the closure condition. If
  the last applied rule is $\m{def}$, since $\clo{\vars'}{V_1 \indv{A_1'} \equiv
  V_2 \indv{A_2'}} \in \mathcal{S}(\mathcal{D}_0)$, we get that $(V_1 \indv{A_1'[\sigma]},
  V_2 \indv{A_2'[\sigma]}) \in \rel$ for any substituion $\sigma$ over $\vars'$.
  The second premise of the $\m{def}$ rule ensures that there exists a substition
  $\sigma'$ over $\vars'$ such that $(V_1 \indv{A_1'[\sigma']}, V_1 \indv{A_1})
  \in \rel$ and $(V_2 \indv{A_2'[\sigma']}, V_2 \indv{A_2}) \in \rel$.
  Since we already know that $(V_1 \indv{A_1'[\sigma']},
  V_2 \indv{A_2'[\sigma']}) \in \rel$, and since $\rel$ is transitive, we get that
  $(V_1 \indv{A_1}, V_2 \indv{A_2}) \in \rel$.

  Further note that extending a relation by its reflexive transitive closure
  preserves its bisimulation properties.
\end{proof}

\subsection{Process for expression server}

To evaluate a term, we can define an \verb`eval` process, parameterized by type \verb`K`.
\begin{verbatim}
decl eval[K] : (t : tm[K]) |- (v : bin * K)
proc v <- eval[K] t =
  case t (
    const =>                % (t : bin * K) |- (v : bin * K)
      n <- recv t ;         % (n : bin) (t : K) |- (v : bin * K)
      send v n ; v <-> t
  | add =>                  % (t : tm[tm[K]]) |- (v : bin * K)
      v1 <- eval[tm[K]] t ; % (v1 : bin * tm[K]) |- (v : bin * K)
      n1 <- recv v1 ;       % (n1 : bin) (v1 : tm[K]) |- (v : bin * K)
      v2 <- eval[K] v1 ;    % (n1 : bin) (v2 : bin * K) |- (v : bin * K)
      n2 <- recv v2 ;       % (n1 : bin) (n2 : bin) (v2 : K) |- (v : bin * K)
      n <- plus n1 n2 ;     % (n : bin) (v2 : K) |- (v : bin * K)
      send v n ; v <-> v2
  | double =>               % (t : tm[K]) |- (v : bin * K)
      v1 <- eval[K] t ;     % (v1 : bin * K) |- (v : bin * K)
      n1 <- recv v1 ;       % (n1 : bin) (v1 : K) |- (v : bin * K)
      n <- double n1 ;      % (n : bin) (v1 : K) |- (v : bin * K)
      send v n ; v <-> v1
  )
\end{verbatim}
The \verb`eval` process uses a channel
\verb`t : tm[K]` as argument,
and offers \verb`v : bin * K`. Intuitively, the process evaluates
term \verb`t` and sends its binary value along \verb`v`. If \verb`t` is a constant, then
\verb`eval[K]` receives the constant $n$, sends it along $v$ and forwards.

The interesting case is the \verb`add` branch. We evaluate the first
summand by spawning a new \verb`eval[K]` process on \verb`t`. Note that since
the type of \verb`t` (indicated on the right) is \verb`tm[tm[K]]`
and hence, the recursive call to \verb`eval` is at parameter  \verb`tm[K]`.
This is in contrast with \emph{nominal polymorphism} in functional
programming languages, where the recursive call must also be at parameter
\verb`K`. We store the value of the first summand at channel \verb`n1 : bin`.
Then, we continue to evaluate the second summand by calling \verb`eval[K]`
on \verb`t` again and storing its value in \verb`n2 : bin`. Finally, we add
\verb`n1` and \verb`n2` by calling the \verb`plus` process, and send the result
\verb`bin` along \verb`v`. We follow a similar approach for the \verb`double`
branch.
